# Supplementary material for: When Private Blockchain Meets Deterministic Database
Source: arXiv:2211.15163 source file (2022-11-28)
Supplement: Supplementary file 1 [file appendix.tex]

\appendix
\section{HarmonyBC with BFT} \label{sec:appendix} 
\added{ ++++move it as the last experiment result}
\added{ ++++the objective and setting are not clear}
HarmonyBC can use a BFT ordering service to tolerate Byzantine faults.
Although BFT consensus protocols are more network-demanding than non-BFT Kafka, we show in the following that 
the BFT version of HarmonyBC can still achieve similar performance as the non-BFT one with a highly optimized BFT consensus protocol (e.g., BFT-SMaRt \cite{bft-smart}).
To do so, we use the same VM cluster as in Section \ref{sec:exp_replica} to evaluate HarmonyBC with BFT-SMaRt as the ordering service. Furthermore, the number of the consensus nodes are scaled up to 80 as we scale the number of replicas.
Figure \ref{fig:bft-smallbank} and Figure \ref{fig:bft-ycsb} shows the results. For comparison, the performance of the non-BFT HarmonyBC obtained in Section \ref{sec:exp_replica} is also shown in the Figures as the dash lines.
The results show that the throughput of HarmonyBC is almost unaffected (less than 5\% drop) with BFT consensus. Since BFT-SMaRt requires more network roundtrips to establish consensus than Kafka, the latency becomes larger and increases with more nodes. However, the increased latency does not affect the end-to-end throughput because BFT-SMaRt is yet the bottleneck even when there up 80 consensus nodes.

\begin{figure}
     \centering
     \includegraphics[width=0.95\linewidth]{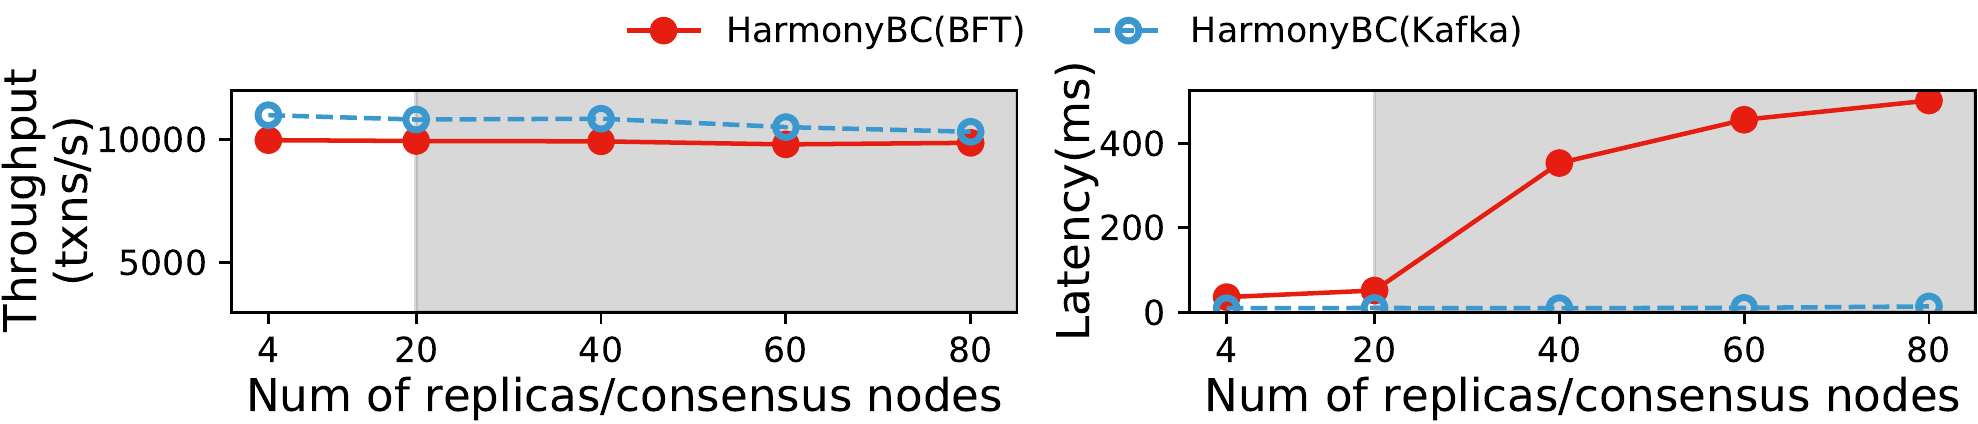}
     \caption{Impact of BFT consensus on smallbank}
     \label{fig:bft-smallbank}
\end{figure}

\begin{figure}
     \centering
     \includegraphics[width=0.95\linewidth]{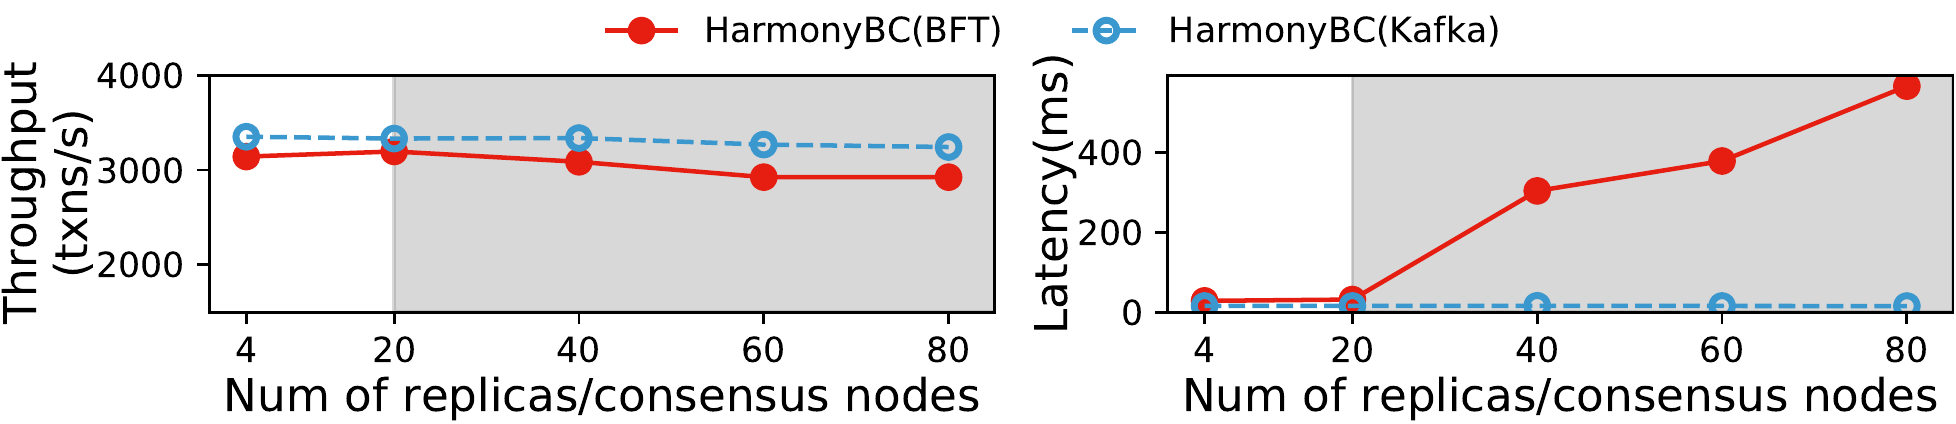}
     \caption{Impact of BFT consensus on YCSB}
     \label{fig:bft-ycsb}
\end{figure}
